# Supplementary material for: Phase-Field Models for Particle-Stabilised Emulsions
Source: arXiv:2602.16622 ancillary file (2026-02-18)
Supplement: Supplementary file 1 [file ESI_arXiv.pdf]

# Electronic Supplementary Information (ESI) for : "Phase-Field Models for Particle-Stabilised Emulsions"

Elisabeth C. Eij,[1,2] Joost de Graaf,[2] Martin F. Haase*,[1] and Jesse M. Steenhoff**[1]

[1)] *Van 't Hoff Laboratory for Physical and Colloid Chemistry, Utrecht University, Utrecht, The Netherlands*

[2)] *Institute for Theoretical Physics, Utrecht University, Utrecht, The Netherlands*

(**j.m.steenhoff@uu.nl)

(*m.f.haase@uu.nl)

This ESI provides additional information to support the findings of the main document. Its content is divided as follows: Section I covers the numerical solution of the dynamic equations presented in this work, which is done *via* finite-volume methods. Section II verifies the behaviour of the immiscible liquids, without any nanoparticles, by characterising their phase separation dynamics. In particular, the late-stage structural evolution of the immiscible liquids is analysed through a power law, extracting the associated coarsening exponents. Section III justifies the chosen relative mobility of the nanoparticles through the Stokes-Einstein-Suntherland equation, in addition to exploring its influence on the coarsening dynamics of the liquid domains. In Section IV, the merger between the phase-field models for STrIPS and particle-stabilised emulsions is elucidated. This includes the dynamic equations and simulation parameters. Finally, Section V provides a more detailed analysis of the size gradients present in the simulated structures of STrIPS bijels.

## I. FINITE-VOLUME SCHEME

### A. Solving the Dynamic Equations

All dynamic equations presented in this work are of the form

$$\frac{\partial \phi}{\partial \tilde{t}} = -\tilde{\nabla} \cdot \tilde{\mathrm{J}}, \tag{1}$$

where $\tilde{\mathrm{J}}$ is the flux of an order parameter $\phi$ that represents a particular component in the system. Considering a general flux driven by a gradient in the chemical potential, $\tilde{\mathrm{J}}$ can be expressed as

$$\tilde{\mathrm{J}} = -\tilde{M}\tilde{\nabla}\tilde{\mu}, \tag{2}$$

with $\tilde{M}$ and $\tilde{\mu}$ the mobility and chemical potential of component $\phi$, respectively. Combining Eqs. (1) and (2) then yields the familiar form of the dynamic equations as shown in the main document

$$\frac{\partial \phi}{\partial \tilde{t}} = \tilde{M}\tilde{\nabla}^2\tilde{\mu} + \tilde{\nabla}\tilde{M} \cdot \tilde{\nabla}\tilde{\mu}. \tag{3}$$

The finite-volume scheme employed in this work evaluates Eq. (1) by discretising the system into a Cartesian grid of $N^d$ cells, with $d$ the dimensionality of the system, and subsequently calculating the cell-averaged divergence of the flux. The following discussion considers the case of a square grid where $d = 2$, but this can be readily adapted for the results with $d = 1$ and $d = 3$ shown in the main document. Figure 1 shows a schematic illustration of the Cartesian grid for $d = 2$, highlighting the central cell labelled with the indices $i$ and $j$. The relevant fluxes for the cells are evaluated at their boundaries, which are located midway between neighbouring centres. For the central cell, the averaged divergence of the flux is given by

$$\left\langle \tilde{\nabla} \cdot \tilde{\mathrm{J}} \right\rangle_{i,j} = \frac{1}{h}\left(\tilde{\mathrm{J}}_{i+1/2,j} + \tilde{\mathrm{J}}_{i,j+1/2} - \tilde{\mathrm{J}}_{i-1/2,j} - \tilde{\mathrm{J}}_{i,j-1/2}\right), \tag{4}$$

where $\tilde{\mathrm{J}}_{i\pm1/2,j}$ and $\tilde{\mathrm{J}}_{i,j\pm1/2}$ are the fluxes normal to the adjacent faces of the cell, while $h$ is the length of each of its sides. For a Cartesian grid, $h$ is also the spacing between the centres of neighbouring cells. In this work, the value of $h$ is generally kept constant at $h = 1$. However, it is changed to $h = 0.5$ for the 1D simulations in Figures 2 and 3 of the main document to better illustrate the liquid interface.

The normal fluxes in Eq. (4) are the result of differences in the chemical potential between adjacent cells. Consequently, they can be assigned by applying a finite-difference approach to the

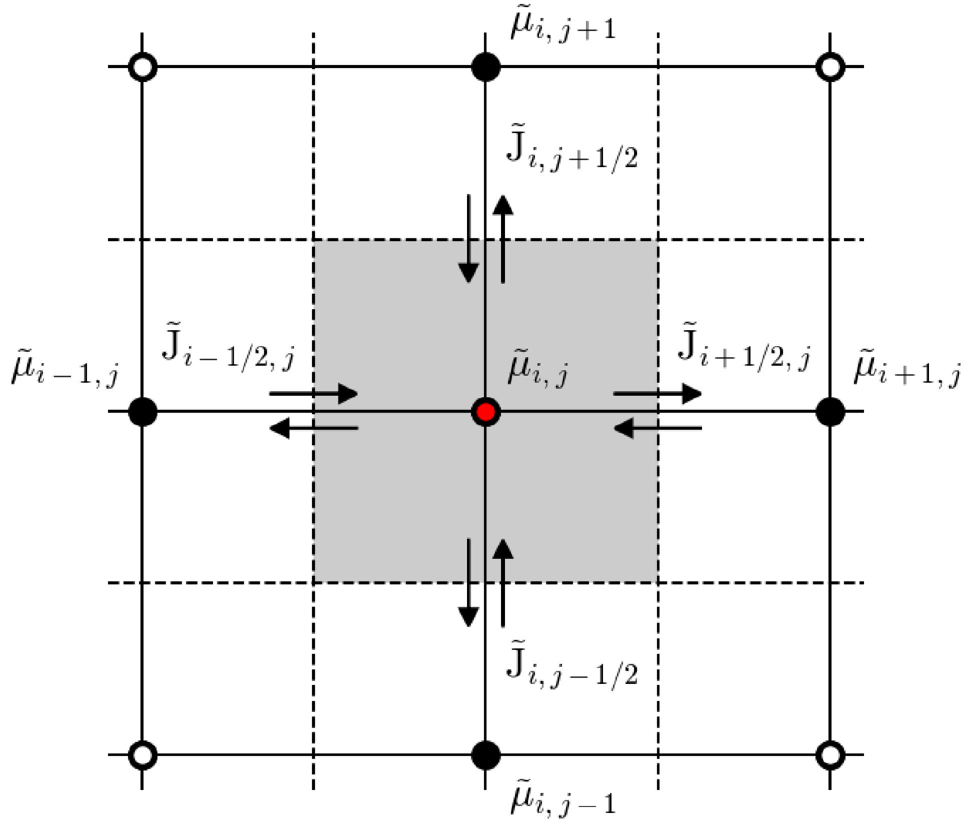


FIG. 1. 2D Cartesian grid used to numerically solve the dynamic equation (1) *via* a finite-volume approach. The central cell, with indices $i$ and $j$, is shaded grey. Its direct neighbours are also shown, with the boundaries between adjacent cells indicated by the dashed lines. The arrows represent the normal fluxes, $\tilde{J}_{i\pm1/2,j}$ and $\tilde{J}_{i,j\pm1/2}$, over these boundaries. Finally, the centres of the cells form a regular lattice that is used for the calculation of the cell-averaged chemical potential $\tilde{\mu}_{i,j}$ through Eqs. (7-10).

chemical potential. For example, the flux over the right boundary of the central cell is given by

$$\tilde{J}_{i+1/2,j} = -\tilde{M}_{i+1/2,j}\left(\frac{\tilde{\mu}_{i+1,j} - \tilde{\mu}_{i,j}}{h}\right), \tag{5}$$

where $\tilde{M}_{i+1/2,j}$ is the local mobility at that boundary. In this work, the local mobility at a boundary is taken to be the harmonic mean of the mobilities of the two bridged cells, so that

$$\tilde{M}_{i+1/2,j} = \frac{2\tilde{M}_{i,j}\tilde{M}_{i+1,j}}{\tilde{M}_{i,j} + \tilde{M}_{i+1,j}}. \tag{6}$$

Subsequently, the cell-averaged chemical potential $\tilde{\mu}_{i,j}$ is determined by treating the centres of the cells as an effective 5-point stencil and using a centred finite-difference for the spatial

discretisation of the required operators. In this case, the chemical potentials of the liquid $\tilde{\mu}^{\phi}_{i,j}$ and the nanoparticles $\tilde{\mu}^{\psi}_{i,j}$ become

$$\tilde{\mu}^{\phi}_{i,j} = \ln \frac{\phi_{i,j}}{1-\phi_{i,j}} + \chi_{i,j}\left(1-2\phi_{i,j}\right) - \tilde{\nabla}^2\phi\big|_{i,j} \; ; \tag{7}$$

$$\tilde{\mu}^{\psi}_{i,j} = \ln \psi_{i,j} - \frac{\tilde{\alpha}}{2}\, |\tilde{\nabla}\phi|^2\big|_{i,j} \; , \tag{8}$$

with $\chi_{i,j}$ and $\tilde{\alpha}$ the interaction and attachment parameters, respectively, while the gradient and Laplacian of the liquid composition $\phi_{i,j}$ are given by

$$\tilde{\nabla}\phi\big|_{i,j} \approx \left(\frac{\phi_{i+1,j}-\phi_{i-1,j}}{2h}, \frac{\phi_{i,j+1}-\phi_{i,j-1}}{2h}\right); \tag{9}$$

$$\tilde{\nabla}^2\phi\big|_{i,j} \approx \frac{\phi_{i+1,j}+\phi_{i-1,j}+\phi_{i,j+1}+\phi_{i,j-1}-4\phi_{i,j}}{h^2}. \tag{10}$$

The combination of Eqs. (4-10) yields the cell-averaged divergence $\langle\tilde{\nabla}\cdot\tilde{\mathrm{J}}\rangle_{i,j}$, which in turn allows the evaluation of the time derivative $\left\langle \frac{\partial\phi}{\partial\tilde{t}} \right\rangle_{i,j}$ through Eq. (1). Finally, the solution $\phi_{i,j}$ is then propagated in time using the Forward Euler approximation. Accordingly, at the time step $n+1$ the solution $\phi^{n+1}_{i,j}$ is calculated through

$$\phi^{n+1}_{i,j} \approx \phi^{n}_{i,j} + \left\langle \frac{\partial\phi}{\partial\tilde{t}} \right\rangle^{n}_{i,j} \Delta\tilde{t}, \tag{11}$$

where $\Delta\tilde{t}$ is the time difference between sequential steps.

## B. Harmonic Mean for the Boundary-Centred Mobility

It is important to emphasise that the harmonic mean in Eq. (6) plays a crucial role for the purposes of the model. That is, the main objective here is to induce structural arrest in a system of two phase-separating liquids by reducing the interfacial mobility between the two bulk phases. In particular, this is achieved by lowering the cell-averaged mobilities in the interfacial region upon accumulation of nanoparticles, reflecting the formation of a jammed particle scaffold.

However, because of the limited width of the interface, there remain plenty of interfacial cells that share boundaries with those in the bulk phases. If the large differences between the cell-averaged mobilities on the interface and in the bulk are not properly accounted for when calculating the boundary-centred mobility, this can cause residual structural coarsening even after the supposed jamming transition has taken place. This is demonstrated in Figure 2, showing the

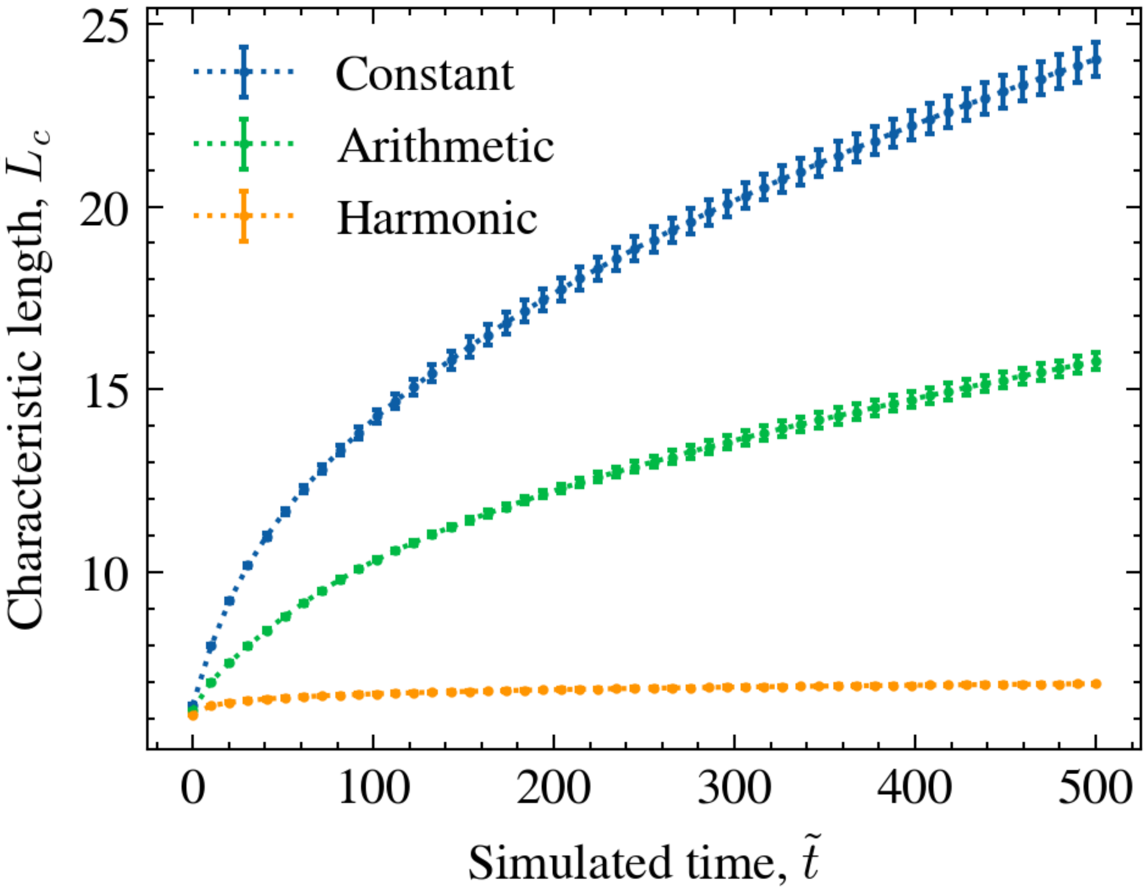


FIG. 2. Change of the characteristic length $\tilde{L}_c$ during the formation of 2D bijels, using different methods to calculate the boundary-centred mobility. The reference employs a constant mobility value, preventing the arrest of phase separation. Compared to this reference, only the harmonic mean of the cell-averaged mobilities $\tilde{M}_{i,j}$ results in full structural arrest after reaching the jamming transition, while the arithmetic mean merely slows down the rate of phase separation. These simulations were further performed with $\psi_0 = 0.50$, $\psi_c = 0.60$ and $\tilde{\alpha} = 60$.

growth of the characteristic length $\tilde{L}_c$ for 2D bijels while using different methods to calculate the boundary-centred mobility.

The profiles in Figure 2 reveal that only the harmonic mean results in full structural arrest after exceeding the jamming threshold. Using an alternative method, such as the arithmetic mean, merely reduces the rate of phase separation. This is because with an arithmetic mean the mobility at the boundary between an interfacial and bulk cell still allows for a significant flux, even if the local mobility of the interfacial cell is close to zero. The harmonic mean in Eq. (6), where the

smaller of the two values dominates, effectively eliminates this issue and achieves proper structural arrest.

### C. Boundary Conditions

The boundary conditions in the system are imposed through both the cell-averaged values and the normal fluxes. For example, periodic boundary conditions along the $i$-indices are enforced through the substitutions $i-1 \to N-1$ and $i+1 \to 0$ in Eqs. (5-6,9-10) for the cells at $i=0$ and $i=N-1$, respectively, while simultaneously equating the fluxes $\tilde{\mathrm{J}}_{-1/2,j} = \tilde{\mathrm{J}}_{N-1/2,j}$ in Eq. (4). For the simulations presented in the main document, a variety of boundary conditions are employed. The 1D and 2D simulations use Neumann ("no-flux") and periodic conditions along all boundaries, respectively. For the boundary conditions of the combined 3D STrIPS model, the reader is referred to Section IV and the original work[1].

## II. ANALYSIS OF LATE-STAGE COARSENING DYNAMICS

In this section, the late-stage coarsening dynamics of the immiscible liquids are analysed. To this end, the evolution of a characteristic length is evaluated over time. Here, the chosen characteristic length depends on the morphology of the liquids, and therefore on the initial composition $\phi_0$.

For the critical composition $\phi_0 = 0.50$ the resulting morphology is bicontinuous. Accordingly, the characteristic length $L_c$ is taken as the inverse of the first moment of the rotationally averaged power spectrum[2–4] $S(k,t)$

$$L_c(t) = 2\pi \frac{\int S(k,t)dk}{\int kS(k,t)dk}, \tag{12}$$

where $S(k,t)$ is given by

$$S(k,t) = \langle \hat{\phi}(\boldsymbol{k},t)\hat{\phi}(-\boldsymbol{k},t)\rangle_k. \tag{13}$$

Here, $\hat{\phi}(\boldsymbol{k},t)$ and $\hat{\phi}(\boldsymbol{k},t)\hat{\phi}(-\boldsymbol{k},t)$ represent the Fourier transform and the power spectrum of the liquid composition $\phi(\boldsymbol{x},t)$, respectively. The outer brackets indicate the rotational average over concentric rings in $\boldsymbol{k}$-space at fixed values of $k$, where $k = |\boldsymbol{k}|$. In contrast, the off-critical composition $\phi_0 = 0.25$ results in a collection of well-dispersed, individual droplets. For this morphology, the droplet diameter is taken as the characteristic length $L_c$, determined *via* the `skimage` package

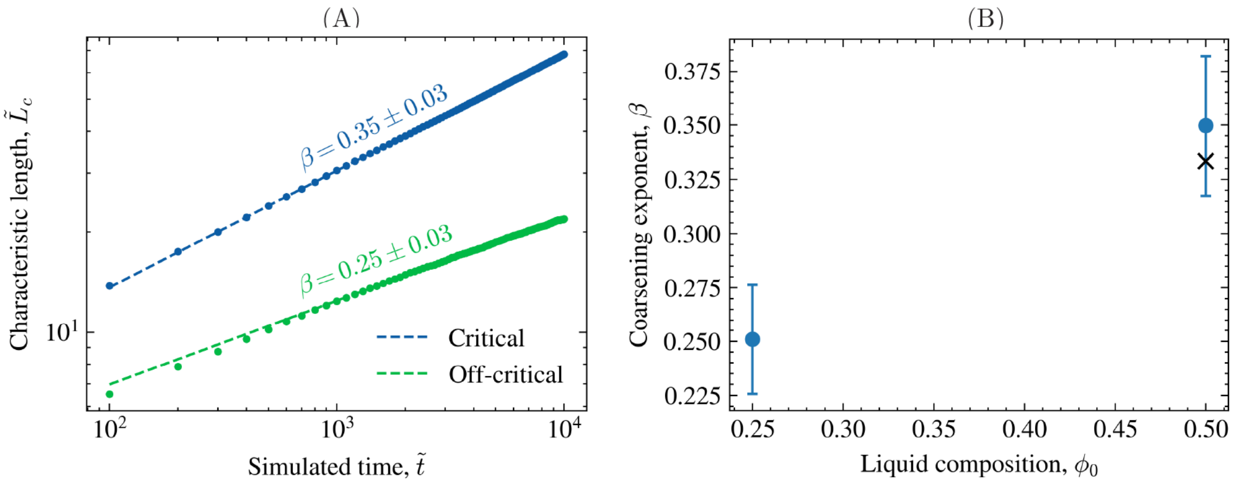


FIG. 3. (A) Profiles showcasing the evolution of the characteristic length $\tilde{L}_c$ over time for critical ($\phi_0 = 0.50$) and off-critical ($\phi_0 = 0.25$) phase separation of the immiscible liquids. (B) Coarsening exponents $\beta$ obtained from fitting the profiles in (A) to a power law. The black cross indicates the theoretical prediction of $\beta = 1/3$ for late-stage coarsening at the critical composition $\phi_0 = 0.50$.

in `Python`. This approach has the advantage of providing the distribution of $L_c$ at any time, rather than a singular value.

The evolution of the characteristic length for both critical and off-critical phase separation is shown in Figure 3A. In both cases, the growth of the characteristic length obeys a power law

$$L_c(t) \propto t^{\beta}, \tag{14}$$

where $\beta$ represents the coarsening exponent.

The value of $\beta$ depends on the initial composition $\phi_0$, as further illustrated in Figure 3B. For critical phase separation at $\phi_0 = 0.50$, the determined $\beta = 0.35 \pm 0.03$ contains the theoretical value of $\beta = 1/3$ predicted by Lifshitz, Slyozov and Wagner[5,6], validating the late-stage coarsening dynamics of the liquids. In contrast, the coarsening kinetics for the off-critical phase separation at $\phi_0 = 0.25$ are noticeably slower. Although this observation is in line with the literature, the calculated value of $\beta = 0.25 \pm 0.03$ is somewhat lower than previously reported[7]. This discrepancy is likely related to the direct measurement of the droplet diameter $L_c$, rather than through Eq. (12), in addition to the comparatively small size ($N = 256$) of the simulated system.

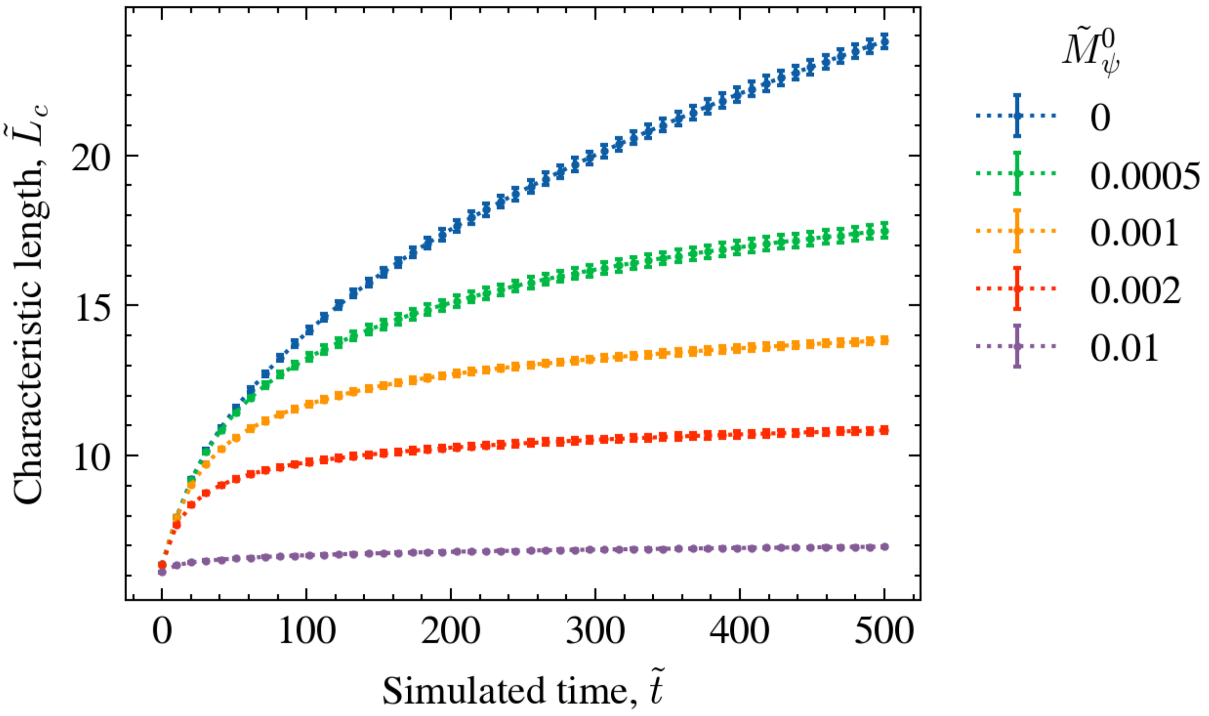


FIG. 4. Evolution of the characteristic length $\tilde{L}_c$ during the formation of 2D bijels with different base mobilities of the nanoparticles $\tilde{M}_\psi^0$. A reference is also included where the nanoparticles are completely stationary, effectively preventing the arrest of phase separation. Apart from the base mobility, other relevant simulation parameters are $\psi_0 = 0.50$, $\psi_c = 0.60$ and $\tilde{\alpha} = 60$.

## III. RELATIVE MOBILITY OF THE NANOPARTICLES

In the main document, the base mobility of the nanoparticles, relative to the molecular liquid, is taken as $\tilde{M}_\psi^0 = M_\psi^0 / M_\phi^0 = 0.01$. This choice is based on an estimate from the Stokes-Einstein-Sutherland equation for the diffusion of spherical particles

$$D_\psi = \frac{k_B T}{6\pi\eta R}, \tag{15}$$

which provides the diffusion constant $D_\psi$ of particles with radius $R$ in a liquid with a dynamic viscosity $\eta$, further involving the absolute temperature $T$ and the Boltzmann constant $k_B$.

The diffusion constant of the particles can then be scaled to that of the liquid medium $D_\phi$, which yields

$$\tilde{D}_\psi = \frac{D_\psi}{D_\phi} = \frac{k_B T}{6\pi R \eta D_\phi}. \tag{16}$$

Taking water as the liquid medium, its diffusion constant and dynamic viscosity at $T = 298$ [K]

are given by $D_\phi = 2.3 \times 10^{-9}$ $[\mathrm{m}^2/\mathrm{s}]$ and $\eta = 0.89 \times 10^{-3}$ $[\mathrm{Pa} \cdot \mathrm{s}]$, respectively. For spherical nanoparticles with radius $R = 10$ [nm], a typical size of the nanoparticles in STrIPS bijels, the relative diffusion constant then becomes

$$\tilde{D}_\psi = \frac{k_B T}{6\pi R \eta D_\phi} \approx 0.01. \tag{17}$$

In the presented model for particle-stabilised emulsions, the arrest of phase separation is driven purely by the kinetics of interfacial nanoparticle accumulation. Consequently, the relative mobility of the nanoparticles has a notable influence on the coarsening dynamics of the liquid domains. This is illustrated in Figure 4, showing the evolution of the characteristic length $\tilde{L}_c$ during the formation of 2D bijels with different values for the base mobility of the nanoparticles $\tilde{M}^0_\psi$. Lower values of $\tilde{M}^0_\psi$ slow down the interfacial accumulation of the nanoparticles, causing phase separation to be arrested at later stages. As visible in the profiles of Figure 4, this results in larger sizes of the stabilised liquid domains.

## IV. EXTENDING THE STRIPS MODEL

This section contains the details regarding the extended phase-field model for bijel formation *via* solvent-transfer induced phase separation (STrIPS), effectively constituting a merger between the pre-existing model for STrIPS[1] and the phase-field framework for particle-stabilised emulsions presented in this work.

The extended STrIPS model introduces a solvent field $\phi_s$ that controls the interaction between the immiscible liquids $\phi$ through the parameter $\chi$. The exact relation between $\phi_s$ and $\chi$ can be found in the original work. At high solvent levels $\phi_s \geq 0.5$ the interaction parameter $\chi \leq 2$, preventing phase separation. Once the solvent diffuses from the precursor, however, the interaction parameter increases and initiates spinodal decomposition of the immiscible liquids. The interfacial attachment of nanoparticles $\psi$ subsequently stabilises the formed emulsion.

In this model, the diffusion of the solvent is simply governed by Fick's second law. Accordingly, effects such as preferential partitioning between the formed liquid phases or imposed diffusion barriers by dense nanoparticle scaffolds are not taken into account. The dynamic equations of the STrIPS system are then given by

$$\frac{\partial \phi_s}{\partial t} = D_s \nabla^2 \phi_s; \tag{18}$$

$$\frac{\partial \phi}{\partial t} = M_\phi(\psi)\nabla^2\mu_\phi + \nabla\mu_\phi \cdot \nabla M_\phi(\psi); \tag{19}$$

$$\frac{\partial \psi}{\partial t} = M_\psi(\psi)\nabla^2\mu_\psi + \nabla\mu_\psi \cdot \nabla M_\psi(\psi), \tag{20}$$

with the diffusion constant of the solvent $D_s$ and the density-dependent mobilities of the immiscible liquids $M_\phi(\psi)$ and nanoparticles $M_\psi(\psi)$. Additionally, the chemical potentials of the latter two components are given by

$$\mu_\phi = f\left(\ln\frac{\phi}{1-\phi} + \chi_s(1-2\phi)\right) - \kappa\nabla^2\phi; \tag{21}$$

$$\mu_\psi = f\ln\psi - \frac{\alpha}{2}|\nabla\phi|^2, \tag{22}$$

where $\chi_s(\phi_s)$ and $\kappa$ are the solvent-mediated interaction and gradient energy parameters of the immiscible liquids, respectively, $f$ is the scale of the free-energy density in the system and $\alpha$ the attachment parameter of the nanoparticles.

Following the original work, the dynamics of the system are scaled with respect to the diffusion of the solvent. Considering diffusion across the interfacial length $\sqrt{\kappa/f}$, the characteristic length $\lambda$ and time $\tau$ are chosen as

$$\lambda = \sqrt{\frac{\kappa}{f}}; \tag{23}$$

$$\tau = \frac{\lambda^2}{D_s} = \frac{\kappa}{fD_s}. \tag{24}$$

With these variables, the nondimensional versions of Eqs. (18), (19) and (20) respectively become

$$\frac{\partial \phi_s}{\partial \tilde{t}} = \tilde{\nabla}^2\phi_s; \tag{25}$$

$$\frac{\partial \phi}{\partial \tilde{t}} = \tilde{M}_\phi(\psi)\tilde{\nabla}^2\tilde{\mu}_\phi + \tilde{\nabla}\tilde{\mu}_\phi \cdot \tilde{\nabla}\tilde{M}_\phi(\psi); \tag{26}$$

$$\frac{\partial \psi}{\partial \tilde{t}} = \tilde{M}_\psi(\psi)\tilde{\nabla}^2\tilde{\mu}_\psi + \tilde{\nabla}\tilde{\mu}_\psi \cdot \tilde{\nabla}\tilde{M}_\psi(\psi), \tag{27}$$

where the nondimensional versions of the chemical potentials $\tilde{\mu}_\phi$ and $\tilde{\mu}_\psi$ are given by

$$\tilde{\mu}_\phi = \ln\frac{\phi}{1-\phi} + \chi_s(1-2\phi) - \tilde{\nabla}^2\phi; \tag{28}$$

$$\tilde{\mu}_\psi = \ln\psi - \frac{\tilde{\alpha}}{2}|\tilde{\nabla}\phi|^2, \tag{29}$$

with $\tilde{\alpha} = \alpha/\kappa$ as the scaled attachment parameter. Additionally, the relative mobilities of the immiscible liquids $\tilde{M}_\phi(\psi)$ and the nanoparticles $\tilde{M}_\psi(\psi)$ follow from

$$\tilde{M}_i(\psi) = \frac{\tilde{M}_i^0}{2}\left(1 - \tanh\left(n\left(\psi - \psi_c\right)\right)\right), \tag{30}$$

where the jamming transition takes place at an interfacial density $\psi_c = 0.60$, with a sharpness parameter $n = 75$. Here, $\tilde{M}_\phi^0$ and $\tilde{M}_\psi^0$ are the base mobilities of the liquids and nanoparticles, respectively, in relation to the solvent. To capture the same relative kinetics of solvent diffusion and phase separation as in the original work, in Eq. (30) the base mobilities of the density-dependent $\tilde{M}_\phi(\psi)$ and $\tilde{M}_\psi(\psi)$ are set to $\tilde{M}_\phi^0 = 10^{-2}$ and $\tilde{M}_\psi^0 = 10^{-4}$, respectively.

For the simulations in Figure 6 of the main document, Eqs. (25), (26) and (27) are numerically solved with $\tilde{\alpha} = 60$ and different initial nanoparticle densities $\psi_0$, starting from the critical composition $\phi^0 = 0.50$ / $\phi_s^0 = 0.50$. Note that $\phi_s$ does not reflect a physical volume fraction here, with more details provided in the original work. Eqs. (26) and (27) are subject to in-plane periodic boundary conditions and "no-flux" conditions at the interface with both the liquid ambient phase and the solid substrate. Although Eq. (25) is also solved with periodic boundary conditions in-plane and a "no-flux" condition at the solid substrate, it has a "flux" condition at the interface with the ambient liquid, which maintains a constant solvent level of $\phi_s = 0$.

## V. DEPTH PROFILE ANALYSIS

The depth profiles in Figure 5A show the evolution of the domain size across the structure of STrIPS bijels. The slopes of these profiles notably vary with depth: starting off steep and flattening out deeper in. Although the depth profiles themselves are smooth, here they are divided into two linear sections to obtain an approximate measure of the slope in the different regions of the bijel structure. The region close to the interface with the ambient liquid is referred to as Region I, while the region deeper in the bijel is called Region II.

Subsequently, the approximate slopes in Regions I and II are obtained from linear fits of the domain size through the respective region, as shown in Figure 5A. The results are reported in Figure 5B, showing the slopes in both regions versus the initial concentration of nanoparticles $\psi_0$. Note that since the depth profiles in Figure 5A are the averages of 25 simulations each, the slopes depicted in Figure 5B are the averages of all individual profiles, rather than the slope of the averaged profile.

Now, there is a notable difference between the slopes of Region I and Region II, with the former steeper than the latter. This observation directly reflects the local solvent gradients that develop during STrIPS, as illustrated in Figure 5C. The asymmetric diffusion of the solvent to the ambient liquid causes higher solvent gradients in Region I than in Region II, enhancing local differences

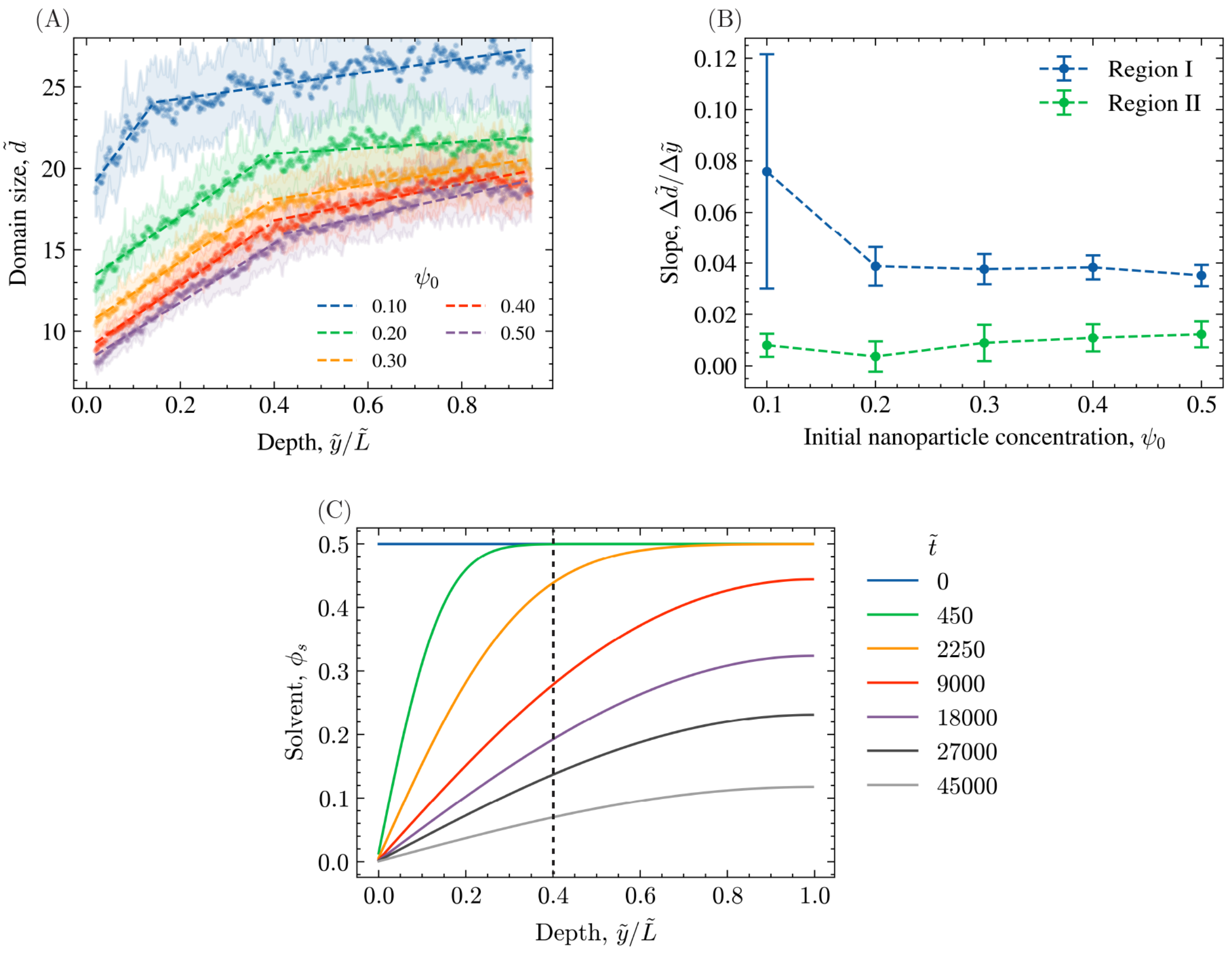


FIG. 5. (A) Profiles of the average domain size over the depth of simulated bijels with $\tilde{L} = 512$, shown for different initial concentrations of the nanoparticles $\psi_0$. The profiles themselves are smooth, yet to acquire an approximate local slope two linear fits are performed over different regions in the bijel structure, represented by the dashed lines. The shaded areas are within a single standard deviation from the average. (B) Slopes of the different regions in the depth profiles of (A). Illustrated is the variation of the slopes for increasing initial nanoparticle concentration $\psi_0$. Region I and Region II refer to the regions close to the ambient liquid and deeper in the bijel structure, respectively. (C) Solvent $\phi_s$ profiles over the bijel structure at different stages of the STrIPS process. These profiles showcase that the asymmetric diffusion into the liquid ambient phase ($\tilde{y}/\tilde{L} = 0$) induces regions with higher and lower solvent gradients. The dashed vertical line gives a rough indication of the boundary between Regions I and II in the bijel structure.

in the rate of phase separation and producing a relatively steep slope in the size of the stabilised domains. In contrast, the flatter solvent profiles in Region II smoothen out local inhomogeneities

in the coarsening rate. The entire region reaches the jamming transition within a narrow time window, yielding a relatively homogeneous distribution in the size of the domains.

Finally, note that for $\psi_0 > 0.10$ the concentration of nanoparticles does not seem to particularly influence the slope of the domain size in the different Regions. Although the slope appears to decrease slightly in Region I with increasing nanoparticle concentration, along with a similar increase in Region II, more extensive investigations in larger systems would be required to make conclusive statements regarding this behaviour. The only notable difference occurs for $\psi_0 = 0.10$, where Region I has a significantly steeper slope and does not extend as deep into the bijel structure. This discrepancy could be related to a regime transition in which the availability of nanoparticles becomes the limiting factor for achieving structural arrest, rather than their accumulation kinetics. However, additional research is needed to validate this claim.

## REFERENCES


[1]J. M. Steenhoff and M. F. Haase, Physical Chemistry Chemical Physics **27**, 5117–5130 (2025).

[2]V. M. Kendon, M. E. Cates, I. Pagonabarraga, J. C. Desplat, and P. Bladon, Journal of Fluid Mechanics **440**, 147–203 (2001).

[3]T. Fujita and M. W. Chen, Japanese Journal of Applied Physics **47**, 1161 (2008).

[4]R. Wittkowski, A. Tiribocchi, J. Stenhammar, R. J. Allen, D. Marenduzzo, and M. E. Cates, Nature Communications **5**, 4351 (2014).

[5]I. M. Lifshitz and V. V. Slyozov, Journal of Physics and Chemistry of Solids **19**, 35–50 (1961).

[6]C. Wagner, Zeitschrift für Elektrochemie, Berichte der Bunsengesellschaft für physikalische Chemie **65**, 581–591 (1961).

[7]B. König, O. J. J. Ronsin, and J. Harting, Physical Chemistry Chemical Physics **23**, 24823–24833 (2021).
